# Supplementary material for: Revisiting Discrete Soft Actor-Critic
Source: arXiv:2209.10081 source file (2024-11-20)
Supplement: Supplementary file 1 [file Appendix_score_raw.tex]

\begin{figure*}[th]
\centering

\includegraphics[width=0.25\textwidth]{images/experiments/over_result_curve_rainbow_sac_rolling_window_length_5/Alien_total.jpeg}
\includegraphics[width=0.25\textwidth]{images/experiments/over_result_curve_rainbow_sac_rolling_window_length_5/Amidar_total.jpeg}
\includegraphics[width=0.25\textwidth]{images/experiments/over_result_curve_rainbow_sac_rolling_window_length_5/Assault_total.jpeg}
\includegraphics[width=0.25\textwidth]{images/experiments/over_result_curve_rainbow_sac_rolling_window_length_5/Asterix_total.jpeg}
\includegraphics[width=0.25\textwidth]{images/experiments/over_result_curve_rainbow_sac_rolling_window_length_5/Asteroids_total.jpeg}
\includegraphics[width=0.25\textwidth]{images/experiments/over_result_curve_rainbow_sac_rolling_window_length_5/BattleZone_total.jpeg}
\includegraphics[width=0.25\textwidth]{images/experiments/over_result_curve_rainbow_sac_rolling_window_length_5/BeamRider_total.jpeg}
\includegraphics[width=0.25\textwidth]{images/experiments/over_result_curve_rainbow_sac_rolling_window_length_5/Breakout_total.jpeg}
\includegraphics[width=0.25\textwidth]{images/experiments/over_result_curve_rainbow_sac_rolling_window_length_5/CrazyClimber_total.jpeg}
\includegraphics[width=0.25\textwidth]{images/experiments/over_result_curve_rainbow_sac_rolling_window_length_5/Enduro_total.jpeg}
\includegraphics[width=0.25\textwidth]{images/experiments/over_result_curve_rainbow_sac_rolling_window_length_5/Freeway_total.jpeg}
\includegraphics[width=0.25\textwidth]{images/experiments/over_result_curve_rainbow_sac_rolling_window_length_5/Frostbite_total.jpeg}
\includegraphics[width=0.25\textwidth]{images/experiments/over_result_curve_rainbow_sac_rolling_window_length_5/Jamesbond_total.jpeg}
\includegraphics[width=0.25\textwidth]{images/experiments/over_result_curve_rainbow_sac_rolling_window_length_5/Kangaroo_total.jpeg}
\includegraphics[width=0.25\textwidth]{images/experiments/over_result_curve_rainbow_sac_rolling_window_length_5/MsPacman_total.jpeg}
\includegraphics[width=0.25\textwidth]{images/experiments/over_result_curve_rainbow_sac_rolling_window_length_5/NameThisGame_total.jpeg}
\includegraphics[width=0.25\textwidth]{images/experiments/over_result_curve_rainbow_sac_rolling_window_length_5/Pong_total.jpeg}
\includegraphics[width=0.25\textwidth]{images/experiments/over_result_curve_rainbow_sac_rolling_window_length_5/Qbert_total.jpeg}
\includegraphics[width=0.25\textwidth]{images/experiments/over_result_curve_rainbow_sac_rolling_window_length_5/SpaceInvaders_total.jpeg}
\includegraphics[width=0.25\textwidth]{images/experiments/over_result_curve_rainbow_sac_rolling_window_length_5/Seaquest_total.jpeg}
\includegraphics[width=0.25\textwidth]{images/experiments/over_result_curve_rainbow_sac_rolling_window_length_5/UpNDown_total.jpeg}
\caption{Learning curves for rainbow, discrere-baseline-SAC and ours, for each individual game. Every curve is smoothed with a moving average of 10 to improve readability.}

\end{figure*}
